# Supplementary material for: Multiphonon transitions in a quantum electromechanical system
Source: arXiv:2108.06241 ancillary file (2021-08-13)
Supplement: Supplementary file 1 [file supplement.pdf]

# Multiphonon transitions in a quantum electromechanical system - Supplementary Information

Alpo Välimaa,[1,*] Wayne Crump,[1,*] Mikael Kervinen,[1,2] and Mika A. Sillanpää[1]

[1]*Department of Applied Physics, Aalto University, P.O. Box 15100, FI-00076 AALTO, Finland*
[2]*Department of Microtechnology and Nanoscience MC2, Chalmers University of Technology, SE-412 96 Göteborg, Sweden*

## I. STARK SHIFT OF THE MULTIPHOTON SPECTRAL LINES

The qubit-oscillator system, where the qubit is driven by a strong transverse field, is described by

$$H = -\frac{\omega_q}{2}\sigma_z + \omega_m(a^\dagger a + 1/2) + g(a^\dagger + a)\sigma_x + \Omega\cos(\omega_{\mathrm{ext}} t)\sigma_x\,. \tag{S1}$$

Here, $\Omega$ is the Rabi frequency, and $\omega_{\mathrm{ext}} \approx \omega_q$ is the frequency of the drive.

In the rotating frame defined by $\omega_{\mathrm{ext}}$, Eq. (S1) becomes

$$H = (\delta - \Delta)\left(a^\dagger a + \frac{1}{2}\right) - \frac{\delta}{2}\sigma_z + g(a^\dagger\sigma^- + a\sigma^+) + \frac{\Omega}{2}\sigma_x\,. \tag{S2}$$

Here, the qubit-drive detuning is $\delta = \omega_q - \omega_{\mathrm{ext}}$, and qubit-oscillator detuning $\Delta = \omega_q - \omega_m$.

Without driving, i.e. $\Omega = 0$, the energies in this frame are those of the Jaynes-Cummings system:

$$E_{\pm,n} = n(\delta - \Delta) \pm \frac{1}{2}\sqrt{4ng^2 + \Delta^2}\,, \quad n \geq 1\,, \tag{S3}$$

and the ground state energy is $E_0 = -\frac{1}{2}\Delta$. The corresponding states, again without driving, are

$$\begin{aligned} |0\rangle &= |g,0\rangle \\ |+,n\rangle &= C|e,n\rangle + S|g,n+1\rangle \\ |-,n\rangle &= -S|e,n\rangle + C|g,n+1\rangle\,. \end{aligned} \tag{S4}$$

In Eq. (S4) and below, we are using a shorthand notation $S = \sin\Theta_n$, $C = \cos\Theta_n$, and $\tan 2\Theta_n = \frac{2g\sqrt{n+1}}{\Delta}$.

The multiquanta transitions based on Eq. (S3) occur if the ground state energy equals those of higher $n$, i.e., $E_{\pm,n} = E_0$. This occurs at the drive detuning

$$\delta_n = \frac{\mp\frac{1}{2}\sqrt{4g^2 n + \Delta^2} - \frac{1}{2}\Delta}{n} + \Delta\,, \tag{S5}$$

or equivalently, when the driving frequency satisfies the condition

$$\omega_{\mathrm{ext}} = \frac{\pm\frac{1}{2}\sqrt{4g^2 n + \Delta^2} + \frac{1}{2}\Delta}{n} + \omega_m\,, \tag{S6}$$

At $\Delta = 0$, Eq. (S5) reduces to

$$\delta_n = \mp\frac{g}{\sqrt{n}}\,. \tag{S7}$$

We now include the driving, $\Omega \neq 0$. Equation (S2) in this case is not analytically solvable any more. We can, however, find approximate results. We work in the bare state basis,

$$\Psi = \sum_{k,l} c_{gk}|g,k\rangle + c_{el}|e,l\rangle\,. \tag{S8}$$

---

[*] equal contribution

Inserting Eq. (S8) into Eq. (S2) results in an infinite matrix, in which we now restrict to the three lowest basis states:

$$\begin{bmatrix} -\frac{1}{2}\Delta & 0 & \frac{1}{2}\Omega \\ 0 & \delta-\frac{3}{2}\Delta & g \\ \frac{1}{2}\Omega & g & \delta-\frac{1}{2}\Delta \end{bmatrix} \begin{bmatrix} c_{g0} \\ c_{g1} \\ c_{e0} \end{bmatrix} = E \begin{bmatrix} c_{g0} \\ c_{g1} \\ c_{e0} \end{bmatrix} . \tag{S9}$$

The driving creates excitations from the ground state to $|e1\rangle$, or, equivalently, to the second Jaynes-Cummings doublet. This renders the system non-blockdiagonal.

Next, we rotate Eq. (S9) to the eigenbasis:

$$H' = UHU^{-1} \tag{S10}$$

with

$$U = \begin{bmatrix} 1 & 0 & 0 \\ 0 & S & C \\ 0 & C & -S \end{bmatrix} . \tag{S11}$$

The result is

$$H' = \begin{bmatrix} -\frac{\Delta}{2} & \frac{1}{2}C\Omega & -\frac{1}{2}S\Omega \\ \frac{1}{2}C\Omega & C^2\left(\delta-\frac{\Delta}{2}\right)+2CSg+S^2\left(\delta-\frac{3\Delta}{2}\right) & C^2g-CS\Delta-gS^2 \\ -\frac{1}{2}S\Omega & C^2g-CS\Delta-gS^2 & C^2\left(\delta-\frac{3\Delta}{2}\right)-2CgS+\frac{1}{2}S^2(2\delta-\Delta) \end{bmatrix} \tag{S12}$$

expressed in the basis $[|0\rangle,\ |-,1\rangle,\ |+,1\rangle]^{\mathrm{T}}$. From Eq. (S12), we can now make an approximation that we select a $2\times 2$ subspace that couples the ground state to either $|-,1\rangle$ or $|+,1\rangle$.

The subspace is determined by if $\delta \geq \Delta$, or the other way round. First we discuss the situation $\delta \geq \Delta$, where the relevant block is that coupling $|0\rangle \Longleftrightarrow |-,1\rangle$:

$$H_2 = \begin{bmatrix} -\frac{\Delta}{2} & -\frac{1}{2}S\Omega \\ -\frac{1}{2}S\Omega & C^2\left(\delta-\frac{3\Delta}{2}\right)-2CSg+\frac{1}{2}S^2(2\delta-\Delta) \end{bmatrix} . \tag{S13}$$

We now treat the resonant condition $\Delta = 0$. Equation (S13) diagonalizes with the energies

$$E_{2,\pm} = \pm\frac{1}{4}\sqrt{(2\delta-2g)^2+2\Omega^2}+\frac{1}{2}\left(\delta-g\right) . \tag{S14}$$

Equation (S14) illustrates how the lowest Jaynes-Cummings doublet is split by the driving. Further, when $\delta = g$ a gap equal to $\Omega/\sqrt{2}$ opens, which means the system undergoes oscillations between the ground state and the first Jaynes-Cummings doublet.

Although Eq. (S2) describes a coupled infinite-level system, we can approximate that the dominant coupling due to the driving is the hybridization of the the levels of $n > 2$ with the energy levels in Eq. (S14). This is illustrated in Fig. 2 in the main text, which also shows how the shift of the multiphoton transitions can be simply pictured as arising from dressing with Eq. (S14). The levels $E_2$ cross the undriven energies $E_{\pm,n}$ as given by Eq. (S3), at a driving frequency that satisfies

$$E_{-,n} = E_{2,+} , \qquad n \geq 2 , \tag{S15}$$

which provides $n$-dependence for the shift.

If $\Delta = 0$, Eq. (S15) reads

$$\delta n - g\sqrt{n} = \frac{1}{4}\sqrt{4(\delta+g)^2+2\Omega^2}+\frac{1}{2}\left(\delta+g\right) , \tag{S16}$$

and yields the positions of the multiphoton resonances:

$$\delta_n^{\Omega} = \frac{\sqrt{4g^2n\left(\sqrt{n}-1\right)^2+2(n-1)n\Omega^2}+2g\sqrt{n}\left(2n-\sqrt{n}-1\right)}{4(n-1)n} \tag{S17}$$

The corresponding shift of the multiphonon resonance due to the driving, up to 4th order in $\Omega$, becomes

$$\epsilon^{\Omega} \equiv \delta_n - \delta_n^{\Omega} \simeq \frac{\Omega^2}{8g\left(n-\sqrt{n}\right)} - \frac{\left(\sqrt{n}+1\right)\Omega^4}{64g^3\left(\sqrt{n}-1\right)^2\sqrt{n}}\ , \qquad n \geq 2 \tag{S18}$$

If $\delta < \Delta$, we consider the block that couples $|0\rangle \Longleftrightarrow |+,1\rangle$. We obtain, similar to Eq. (S13):

$$H_2 = \begin{bmatrix} -\frac{\Delta}{2} & \frac{C\Omega}{2} \\ \frac{C\Omega}{2} & C^2\left(\delta-\frac{\Delta}{2}\right)+2CgS+S^2\left(\delta-\frac{3\Delta}{2}\right) \end{bmatrix} . \tag{S19}$$

In the resonant situation $\Delta = 0$, we obtain from Eq. (S19) the energies

$$E_{2,\pm} = \pm\frac{1}{4}\sqrt{(2\delta+2g)^2+2\Omega^2}+\frac{1}{2}\left(\delta+g\right)\ , \tag{S20}$$

and the multiphoton resonances become, by symmetry, those in Eq. (S17) but with a minus sign in front.

### A. Analytical solutions, $\Delta \neq 0$

Next we collect analytical solutions for arbitrary $\Delta$ in four different situations depending on the signs of $\delta$ and $\Delta$. There are two sets of energy levels from the TLS approximation, Eqs. (S13,S19), given as

$$E^{-}_{2,\pm} = \frac{1}{4}\left(2\delta-\Delta\cos 2\Theta-3\Delta-2g\sin 2\Theta \pm \sqrt{(-2\delta+\Delta\cos 2\Theta+\Delta+2g\sin 2\Theta)^2+4\Omega^2\sin^2\Theta}\right)\ , \tag{S21}$$

$$E^{+}_{2,\pm} = \frac{1}{4}\left(2\delta+\Delta\cos 2\Theta-3\Delta+2g\sin 2\Theta \pm \sqrt{(2\delta+\Delta\cos 2\Theta-\Delta+2g\sin 2\Theta)^2+4\Omega^2\cos^2\Theta}\right) \tag{S22}$$

Let us use a shorthand notation:

$$\begin{aligned} \Delta_{gn} &= \sqrt{4g^2n+\Delta^2} \\ \Delta_{g1} &= \sqrt{4g^2+\Delta^2} \end{aligned} \tag{S23}$$

#### 1. $\Delta \geq 0$, $\delta \geq \Delta$

TLS energies are given by $E^{-}_{2,+}$ in Eq. (S21), and the positions of the multiquanta resonances satisfy

$$\begin{aligned} 4(n-1)n\delta_n^{\Omega} =& \sqrt{2\Delta^2\left(1-(n-1)n\left(\frac{\Delta_{g1}}{\Delta}-1\right)\right)+2\left(-n\frac{\Delta_{g1}}{\Delta}+n-1\right)\Delta\Delta_{gn}+4(n-1)n\Omega^2\sin^2\frac{\Theta}{2}+4g^2n(n+1)} \\ &-\Delta n\left(\frac{\Delta_{g1}}{\Delta}+5\right)+\Delta_{gn}(2n-1)+\Delta(4n^2+1) \end{aligned} \tag{S24}$$

#### 2. $\Delta \geq 0$, $\delta < \Delta$

TLS energies given by $E^{+}_{2,-}$ Eq. (S22).

$$\begin{aligned} 4(n-1)n\delta_n^{\Omega} =& -\sqrt{2\Delta^2\left((n-1)n\left(\frac{\Delta_{g1}}{\Delta}+1\right)+1\right)-2\left(n\frac{\Delta_{g1}}{\Delta}+n-1\right)\Delta\Delta_{gn}+4(n-1)n\Omega^2\cos^2\frac{\Theta}{2}+4g^2n(n+1)} \\ &+\Delta n\left(\frac{\Delta_{g1}}{\Delta}+4n-5\right)+\Delta_{gn}(1-2n)+\Delta \end{aligned} \tag{S25}$$

### *3.* $\Delta < 0$, $\delta > \Delta$

TLS energies given by $E^{+}_{2,+}$ Eq. (S22).

$$4(n-1)n\delta_n^{\Omega} = \sqrt{2\Delta^2\left((n-1)n\left(\frac{\Delta_{g1}}{\Delta}+1\right)+1\right)+2\left(n\frac{\Delta_{g1}}{\Delta}+n-1\right)\Delta\Delta_{gn}+4(n-1)n\Omega^2\cos^2\frac{\Theta}{2}+4g^2n(n+1)} + \Delta n\left(\frac{\Delta_{g1}}{\Delta}+4n-5\right)+\Delta_{gn}(2n-1)+\Delta \tag{S26}$$

### *4.* $\Delta < 0$, $\delta < \Delta$

TLS energies given by $E^{-}_{2,-}$ Eq. (S21).

$$4(n-1)n\delta_n^{\Omega} = -\sqrt{2\Delta^2\left(1-(n-1)n\left(\frac{\Delta_{g1}}{\Delta}-1\right)\right)+2\left(n\frac{\Delta_{g1}}{\Delta}-n+1\right)\Delta\Delta_{gn}+4(n-1)n\Omega^2\sin^2\frac{\Theta}{2}+4g^2n(n+1)} - \Delta n\left(\frac{\Delta_{g1}}{\Delta}+5\right)+\Delta_{gn}(1-2n)+\Delta(4n^2+1) \tag{S27}$$
